# Supplementary material for: Model-Free Active Exploration in Reinforcement Learning
Source: arXiv:2407.00801 source file (2024-06-30)
Supplement: Supplementary file 1 [file full_related_work.tex]

\section{Related Work}\label{sec:full_related_work}
\hl{Move it after the results? check that PSRL is mentioned}
The body of work concerning exploration methods in RL problems is vast, and for simplicity, we strictly focus on online discounted MDPs (for the generative setting one can refer to  the analysis in \cite{gheshlaghi2013minimax,al2021adaptive}).
Most RL exploration strategies draw inspiration from classical multi-armed bandit models \cite{lattimore2020bandit,sutton2018reinforcement}, which include simple techniques as  $\epsilon$-greedy exploration  and  Boltzmann exploration\cite{watkins1989learning, sutton2018reinforcement,lattimore2020bandit,atkins2014atkins}, or more advanced procedures that tries to tackle the parametric uncertainty (\emph{a.k.a.} epistemic uncertainty) \cite{moerland2017efficient} in the parameters, such as Upper-Confidence Bounds (UCB) methods \cite{auer2002using,auer2002finite,lattimore2020bandit} or Bayesian approaches such as Thompson Sampling (TS) methods \cite{thompson1933likelihood,wyatt1998exploration,dearden1998bayesian,russo2018tutorial}. 
We begin by discussing the related work for RL problems in the tabular setting, and later extend the discussion to large state-action spaces that necessitate the use of neural architectures.

\paragraph{Known bounds in tabular Reinforcement Learning (RL).} Herein, due to the amount of literature, we do not discuss the details of the various methods, and only layout what are the known bounds of the algorithms. To the best of our knowledge,  the known lower bound in the minimax setting is $\tilde \Omega\left(\frac{|S||A|}{\varepsilon^2(1-\gamma)^3}\right)$ \cite{lattimore2012pac}\footnote{Logarithmic factors are hidden for simplicity.}, whereas for instance-specific bounds it is known  the best-policy identification (BPI) lower bound in \cite{marjani2021navigating}, which holds solely for MDPs with a unique optimal policy (their method draws inspiration  from the best-arm identification setting with fixed confidence in \cite{garivier2016optimal}).
Various algorithms have been proposed throughout the last decades to try to reach the  lower bounds. Successful model-free approaches \cite{dong2019q,jin2018q} are known for their UCB-like exploration \cite{auer2002using,lattimore2020bandit}, whereas model-based approaches (which require the agent to be able to compute the optimal greedy value function through value iteration) make use of the knowledge of the MDP to guide exploration.
Some of the most known model-free algorithms include \textsc{R-MAX} \cite{kakade2003sample}, \textsc{Delayed Q-Learning} \cite{strehl2006pac} and \textsc{Q-UCB} \cite{dong2019q}.  These algorithms scale, respectively, as with  $\tilde O\left(\frac{|S|^2|A|}{\varepsilon^3(1-\gamma)^6}\right), \tilde O\left(\frac{|S||A|}{\varepsilon^4(1-\gamma)^8}\right)$  and $\tilde O\left(\frac{|S||A|}{\varepsilon^2(1-\gamma)^7}\right)$.
On the other hand, known model-based algorithms include \textsc{MBIE} \cite{strehl2008analysis}, \textsc{MORMAX} \cite{szita2010model} and \textsc{UCRL} \cite{lattimore2012pac}, which scale, respectively, as $ \tilde O\left(\frac{|S|^2|A|}{\varepsilon^3(1-\gamma)^6}\right), \tilde O\left(\frac{|S||A|}{\varepsilon^2(1-\gamma)^6}\right)$ and $\tilde O\left(\frac{|S|^2|A|}{\varepsilon^3(1-\gamma)^3}\right)$. More recently, \cite{marjani2021navigating} proposed \textsc{MDP-NaS}, a model-based approach able to reach the instance-specific lower bound for BPI.

\paragraph{Exploration in Deep Reinforcement Learning (DRL).} Exploration strategies in DRL environments faces several challenges, from the fact that the state-action space is often continuous, to the several problems that practitioners experience when training deep neural architectures (the reader can refer to \cite{sewak2019deep} for a wide range of techniques used to address these challenges). 
The main issue in these large state-action MDPs lies in the fact that good exploration becomes extremely hard when the either the reward is sparse/delayed \cite{yang2021exploration} or the observations contain distracting features (\emph{a.k.a. Noisy-TV} problem \cite{burda2018exploration,yang2021exploration}). 
Sparse rewards makes the learning process more problematic, since networks are prone to forgetting and thus may require several training iterations, whereas distracting features may lead to an increased training time (due to the fact that the network needs to learn how to interpret these features).
Apart from the basic techniques we previously mentioned, there are some other heuristics that are widely used, such as (i) adding an entropy term to the optimization problem to encourage the policy to be more aleatoric \cite{mnih2016asynchronous} (and/or explore in those parts of the state-action space where it is unclear what the optimal action is \cite{haarnoja2018soft}) or (2) injecting noise in the observations/parameters \cite{fortunato2017noisy,plappert2017parameter} (see also \cite{yang2021exploration} for a review).
However, most techniques that try to tackle the exploration problem fall mainly into 2 categories \cite{yang2021exploration}: \emph{uncertainty-based} and \emph{intrinsic-motivation-based} \cite{yang2021exploration,ladosz2022exploration}. Usually, uncertainty-based methods  decouple the uncertainty into {\it epistemic/parametric} and {\it aleatoric} uncertainty. 
Epistemic uncertainty \cite{dearden1998bayesian,moerland2017efficient,kirschner2018information,yang2021exploration} quantifies the uncertainty in the parameters of the state-action value (an example is the posterior distribution of the $Q$-values) that vanishes as the agent explores and learns, while aleatoric uncertainty accounts for the inherent randomness of the environment due to the transition and reward distributions, and the randomness in the policy \cite{moerland2017efficient,kirschner2018information,yang2021exploration}. 
Epistemic uncertainty can be tackled using OFU-like mechanisms, that perform optimistic action-selection on the $Q$-values (for example, by using bounds derived from the posterior of the $Q$-values \cite{osband2013more,chen2017ucb,yang2021exploration}), or TS techniques  that sample from the posterior of the $Q$-values \cite{yang2021exploration}. However, computing a posterior of the $Q$-values is not always possible.
Parametric approaches include  Randomized Least-Squares
Value Iteration (RLSVI) \cite{osband2016generalization} for linear MDPs, which  samples from a Gaussian posterior distribution the action-value function  (similarly, \textsc{PSRL} \cite{osband2013more} samples from a posterior over MDPs). This technique is later extended in Bayesian DQN \cite{azizzadenesheli2018efficient} where the authors use the idea to consider the features before the output layer of the deep-Q network as a fixed feature vector in order to recast the problem as a linear MDP problem. 
Other techniques perform non-parametric posterior sampling by using methods like bootstrapping \cite{osband2015bootstrapped,osband2016deep}. Bootstrapped DQN (and Bootstrapped DQN with prior functions) \cite{osband2016deep,osband2018randomized,osband2019deep} maintains several independent $Q$-value functions, and randomly samples one of them to explore the environment (to date Bootstrapped DQN has become a common
baseline for deep exploration \cite{yang2021exploration}).
%This method takes inspiration from \textsc{RLSVI} \cite{osband2016generalization}, an algorithm that samples from a Gaussian posterior distribution over value functions (similarly, \textsc{PSRL} \cite{osband2013more} samples from a posterior over MDPs).
Subsequently, bootstrapped DQN was extended to consider uncertainty propagation by performing backward induction \cite{bai2021principled}. In \cite{lee2021sunrise} the authors introduce \textsc{SUNRISE}, an algorithm that integrates Bootstrapped DQN with an UCB-like bonus for optimistic action selection (akin to \cite{chen2017ucb} ), and additionally adopts a weighted Bellman update to reduce instability in error propagation in the $Q$-values. For the sake of brevity, we refer to the reader to the survey in \cite{yang2021exploration} for an exhaustive list of algorithms.
However, most of these algorithms do not directly account for  aleatoric uncertainty, which is usually estimated by modeling the distribution of returns.  Thus, algorithms that estimate the aleatoric uncertainty include, for example, Distributional RL approaches \cite{bellemare2017distributional,dabney2017distributional,mavrin2019distributional}. 
Well-known exploration methods that account for both aleatoric and epistemic uncertainties include Double Uncertain Value Network (DUVN) \cite{moerland2017efficient} and Information Directed Sampling  (IDS) \cite{kirschner2018information,nikolov2018information}. The former uses Bayesian dropout to measure the epistemic uncertainty, and the latter uses distributional RL \cite{bellemare2017distributional} to estimate the variance of the returns, and bootstrapped DQN to estimate the epistemic uncertainty in the form of a bound on the estimate of the suboptimality gaps. These quantities are later on combined to compute an information ratio that is used to sample the next action. 
Similarly, in \cite{clements2019estimating} the authors propose \textsc{UA-DQN}, an approach that uses \textsc{QR-DQN} \cite{dabney2017distributional} to learn the epistemic and aleatoric uncertainties from the quantile networks.
Finally, another class of exploration strategy is the class of intrinsic-motivation based methods \cite{ryan2000intrinsic,barto2013intrinsic} These methods assign an intrinsic reward according to different heuristics: estimate prediction errors, state novelty and information gain. However, since these methods are not strictly related to the work herein presented, we refer the reader to \cite{yang2021exploration} for an exhaustive description.
