# Supplementary material for: Model-Free Active Exploration in Reinforcement Learning
Source: arXiv:2407.00801 source file (2024-06-30)
Supplement: Supplementary file 2 [file forced_mfbpi.tex]

\begin{algorithm}[t]\label{algo:obpi}
	\caption{\textsc{MF-BPI}}
	\begin{algorithmic}[1]
		\REQUIRE Parameters $(\varepsilon, \bar k)$ and learning rates $\{(\alpha_t,\beta_t)\}_t$.
		%\smallskip
		\STATE Initialize $\omega_o^{(1)}\gets 1/|S||A|$,  $N_t$,  $Q_1(s,a)\gets 0$ and $M_{1}(s,a)\gets 0$ for all $(s,a)\in S\times A$.
		\STATE Observe $s_0\sim p_0$ and update $N_t$.
		\FOR{$t=0,1,2,\dots,$}
		\STATE Let $\omega^{(t)}(s_t,a) =  \dfrac{\epsilon_t}{|A|} +(1-\epsilon_t)\frac{\omega_o^{(t)}(s_t,a)}{\sum_{a'} \omega_o^{(t)}(s_t,a')} $ be the policy at time $t$ in state $s_t$.
		\STATE Sample $a_t\sim \omega^{(t)}(s_t,\cdot)$; observe $(r_t,s_{t+1})\sim q(\cdot|s_t,a_t)\otimes P(\cdot|s_t,a_t)$ and update $N_t$.
		\STATE Update the $Q$-values and the $M$-values using \cref{eq:stochastic_approximation_step_qvalues,eq:stochastic_approximation_step_mvalues}.
		\STATE Compute  allocation  $\omega_o^{(t+1)}$ in \cref{eq:upper_bound_time_t}.
		\ENDFOR
	\end{algorithmic}
\end{algorithm}
