# Supplementary material for: Model-Free Active Exploration in Reinforcement Learning
Source: arXiv:2407.00801 source file (2024-06-30)
Supplement: Supplementary file 3 [file characteristic_time_convexity_figure.tex]

\begin{figure}[t]
	\centering
	\begin{tikzpicture}
	\begin{axis}[
	axis lines=middle,
	x label style={at={(axis description cs:.5,-0.01)},anchor=north},
	y label style={at={(axis description cs:-0.01,.5)},rotate=90,anchor=south},
	xlabel={Instances $\phi$},
	ylabel={Characteristic time},
	ytick=\empty,
	xmin=0, xmax=10,
	ymin=0, ymax=20,
	domain=0:10,
	samples=100,
	xtick=\empty,
	ytick=\empty,
	legend pos=outer north east
	]

	\addplot[white,thick,name path=G] {sin(deg(x))+x+4}; % plot T^*(M)
	\addplot[black,thick,dashed,name path=U] {sin(deg(x))+x+6}  node[pos=0.9, above]{$U_\varepsilon^\star(\phi)$}; % plot U^*(M)
	\addplot[black,thick,name path=T] {sin(deg(x))+x+2} node[pos=0.95, below]{$T_\varepsilon^\star(\phi)$}; % plot T^*(M)
	\path[name path=axis] (axis cs:0,0) -- (axis cs:10,0);
	\addplot[black!20,pattern=north east lines, pattern color=black!20] fill between[of=G and T,soft clip={domain=0:10}, reverse=true];
	\node (nonconvex) at (axis cs:6, 3) {Non-convex region};
	\draw[->] (nonconvex) -- (axis cs:4,6);
	\end{axis}
	\end{tikzpicture}

   \caption{Computing the lower bound $ T_\varepsilon^\star(\phi)$ is a non-convex problem. Therefore it may not be always possible to approximately solve it. An alternative way is to find an upper bound $\bar U_\varepsilon^\star(\phi)=\min_\omega \bar U_\varepsilon(\omega)$ by convexifying the problem.}
   \label{fig:convexification_lower_bound}
\end{figure}
